# Supplementary material for: Event reconstruction for KM3NeT/ORCA using convolutional neural networks
Source: arXiv:2004.08254 source file (2020-04-17)
Supplement: Supplementary file 1 [file appendix.tex]

\section{Energy reconstruction}

\subsection{Neutral-current events}

\begin{figure}[h!]
	\centering \includegraphics[width=0.675\textwidth,
          page=3]{img/regression/energy/energy_reco_2d_dl.pdf}
	\caption{Reconstructed energy vs. true energy of the deep
          learning reconstruction for $\nu_e-NC$ events.}
	\label{fig:regr_2d_energy_dl_nu_e_nc}
\end{figure}

\begin{figure}[h!]
	\centering \includegraphics[width=0.675\textwidth,
          page=3]{img/regression/energy/energy_reco_2d_std.pdf}
	\caption{Reconstructed energy vs. true energy of the standard
          ORCA reconstruction for $\nu_e-NC$ events.}
	\label{fig:regr_2d_energy_std_nu_e_nc}
\end{figure}

\newpage
\clearpage

\begin{figure}[h!]
	\centering \includegraphics[width=0.675\textwidth,
          page=3]{img/regression/energy/energy_reco_1d_comparison_median_dl_std.pdf}
	\caption{True energy versus the median relative error for
          $\nu_e-NC$ events and both the deep learning as well as the
          standard likelihood-based approach.}
	\label{fig:regr_1d_energy_median_nu_e_nc}
\end{figure}

\begin{figure}[h!]
	\centering \includegraphics[width=0.675\textwidth,
          page=3]{img/regression/energy/energy_reco_1d_comparison_rel_std_dl_std.pdf}
	\caption{True energy versus the relative standard deviation
          for $\nu_e-NC$ events and both the deep learning as well as
          the standard likelihood-based approach.}
	\label{fig:regr_1d_energy_rsd_nu_e_nc}
\end{figure}

\newpage
\clearpage

\section{Direction reconstruction}

\subsection{$\nueCC$ events}

% --- DIRECTION RECONSTRUCTION NU_E_CC

$\nu_e-CC$ azimuth:

\begin{figure}[h!]
	\centering \includegraphics[width=0.675\textwidth, page=2]{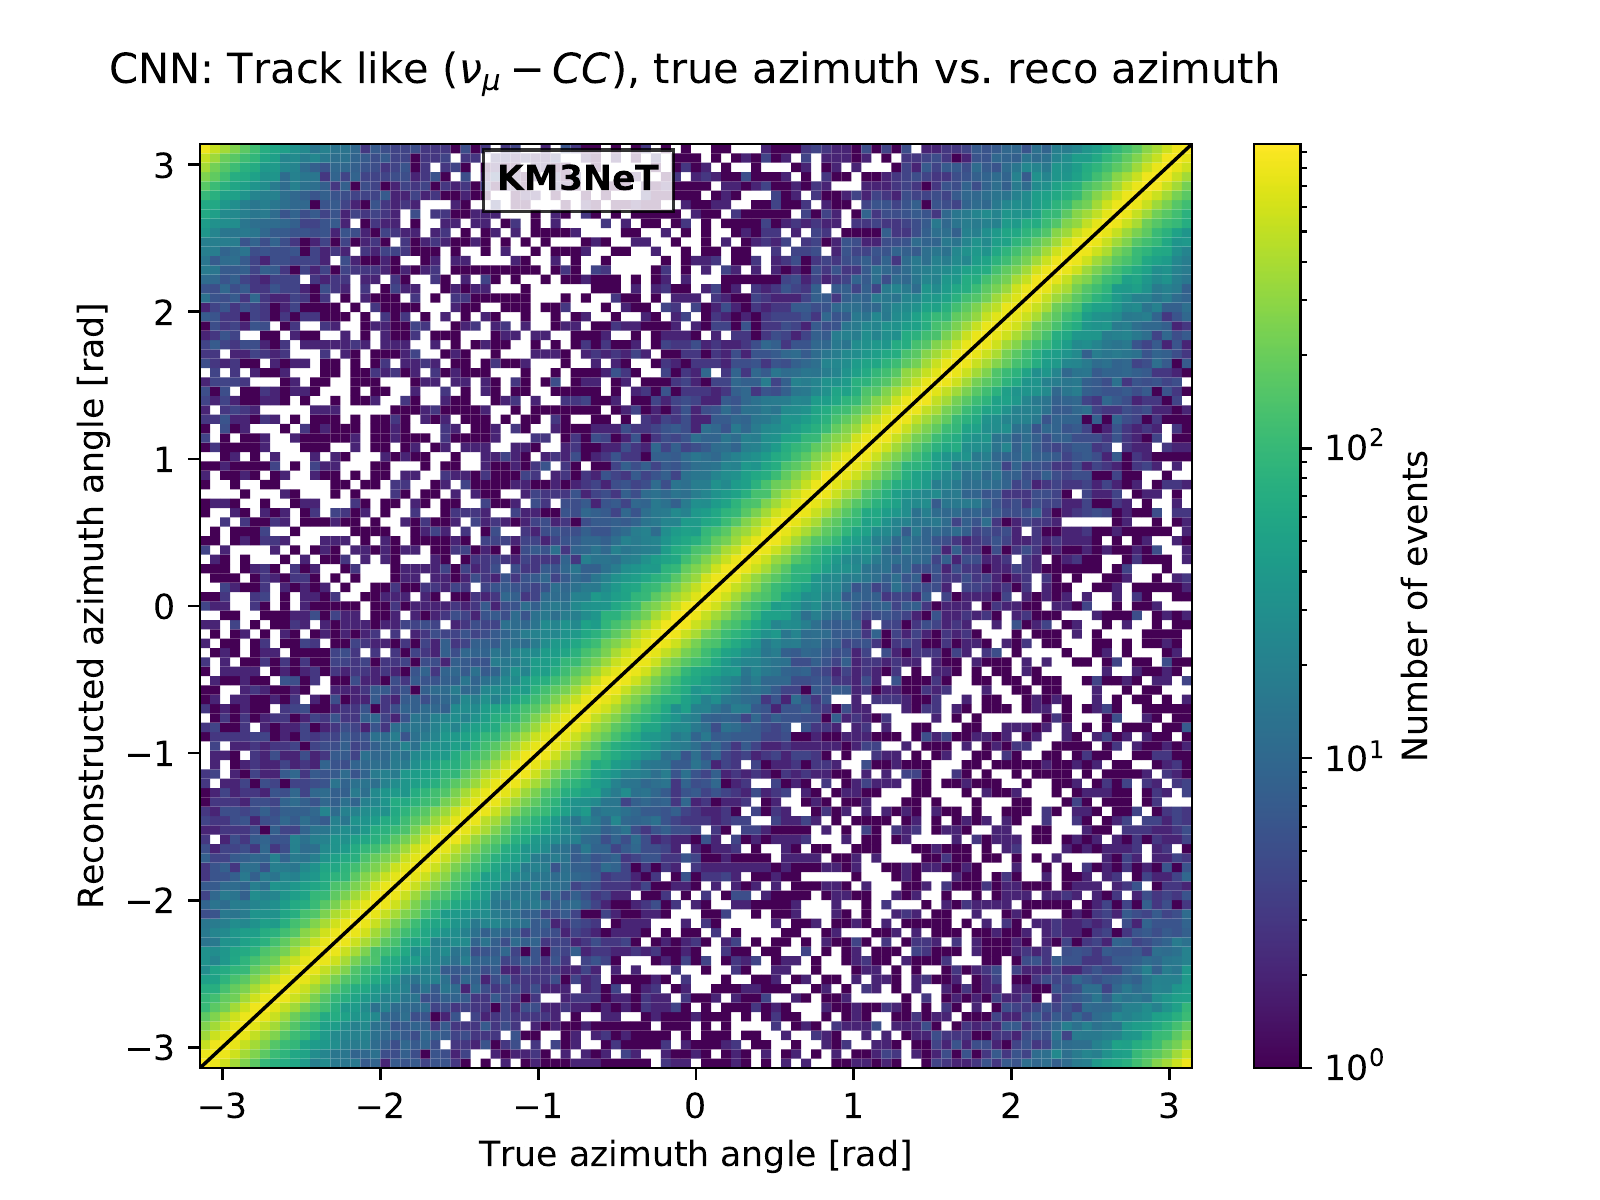}
	\caption{Reconstructed azimuth vs. true azimuth of the deep learning reconstruction for $\nu_e-CC$ events.}
	\label{fig:regr_2d_azimuth_dl_nu_e_cc}
\end{figure}

\begin{figure}[h!]
	\centering \includegraphics[width=0.675\textwidth, page=2]{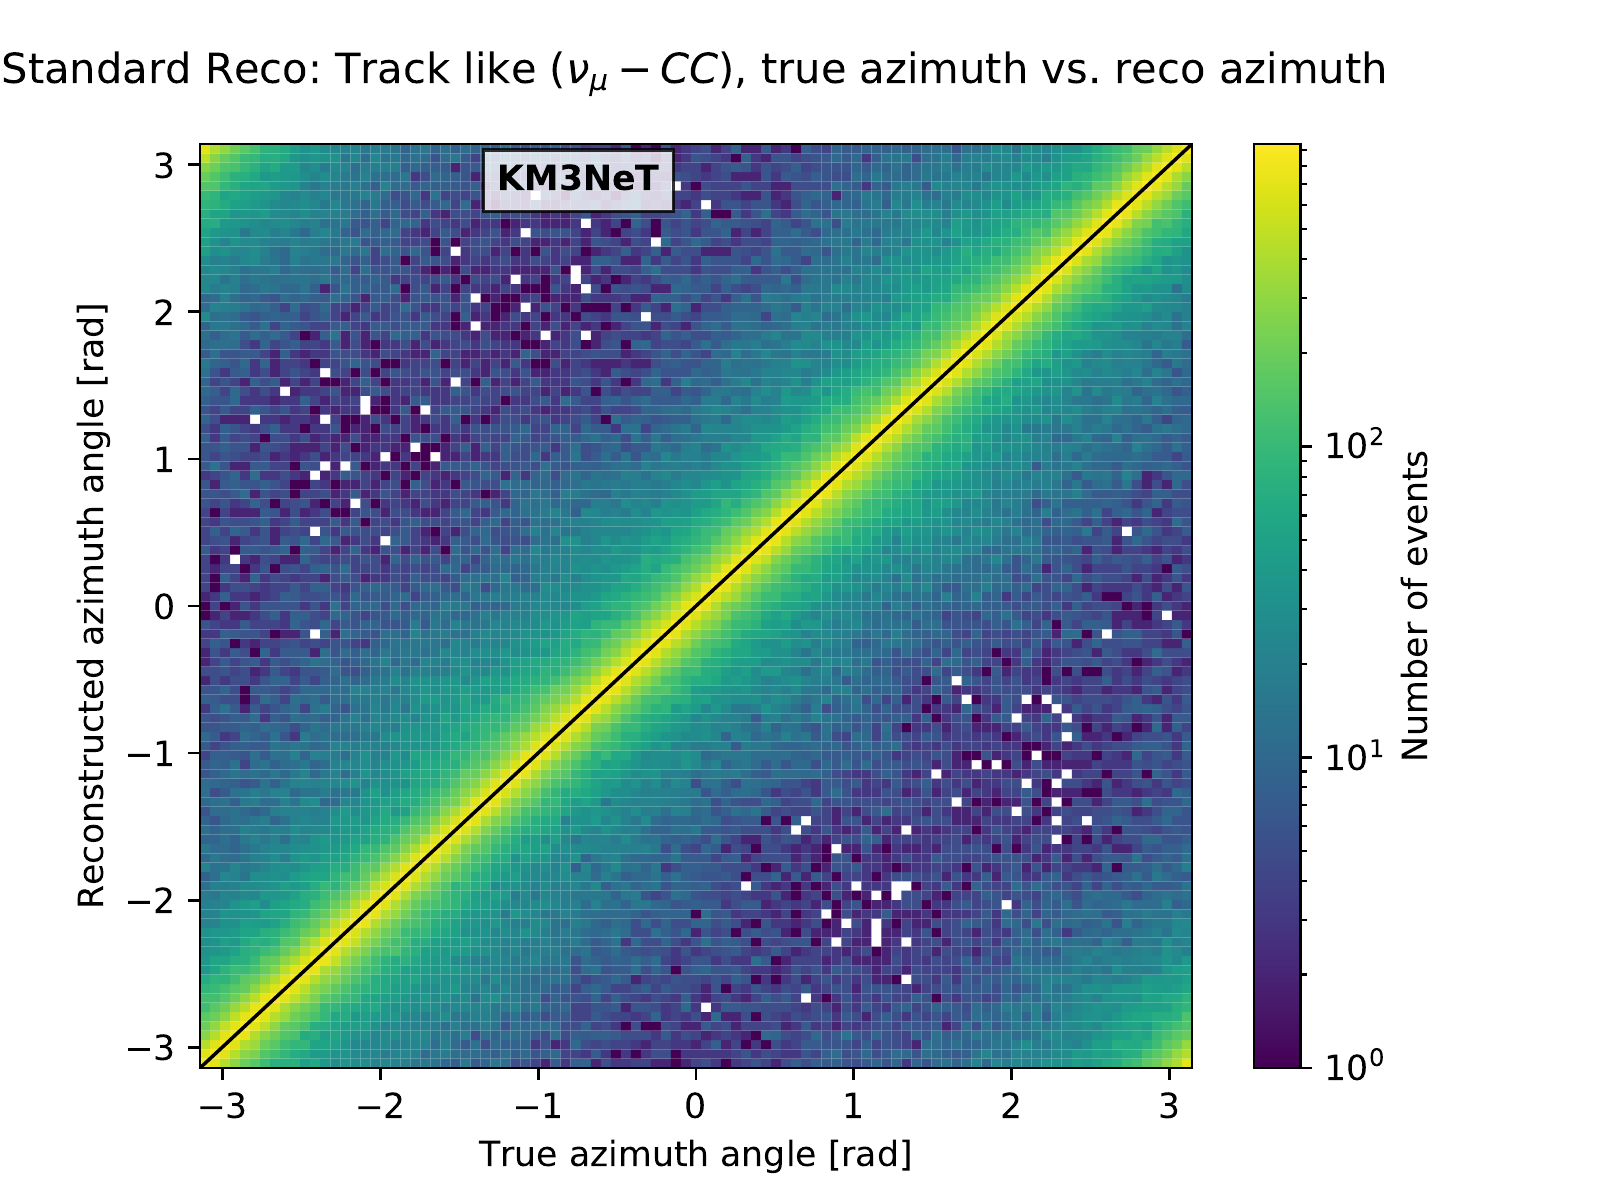}
	\caption{Reconstructed azimuth vs. true azimuth of the standard, likelihood-based ORCA reconstruction for $\nu_e-CC$ events.}
	\label{fig:regr_2d_azimuth_std_nu_e_cc}
\end{figure}

\newpage
\clearpage

$\nu_e-CC$ zenith:

\begin{figure}[h!]
	\centering \includegraphics[width=0.675\textwidth, page=2]{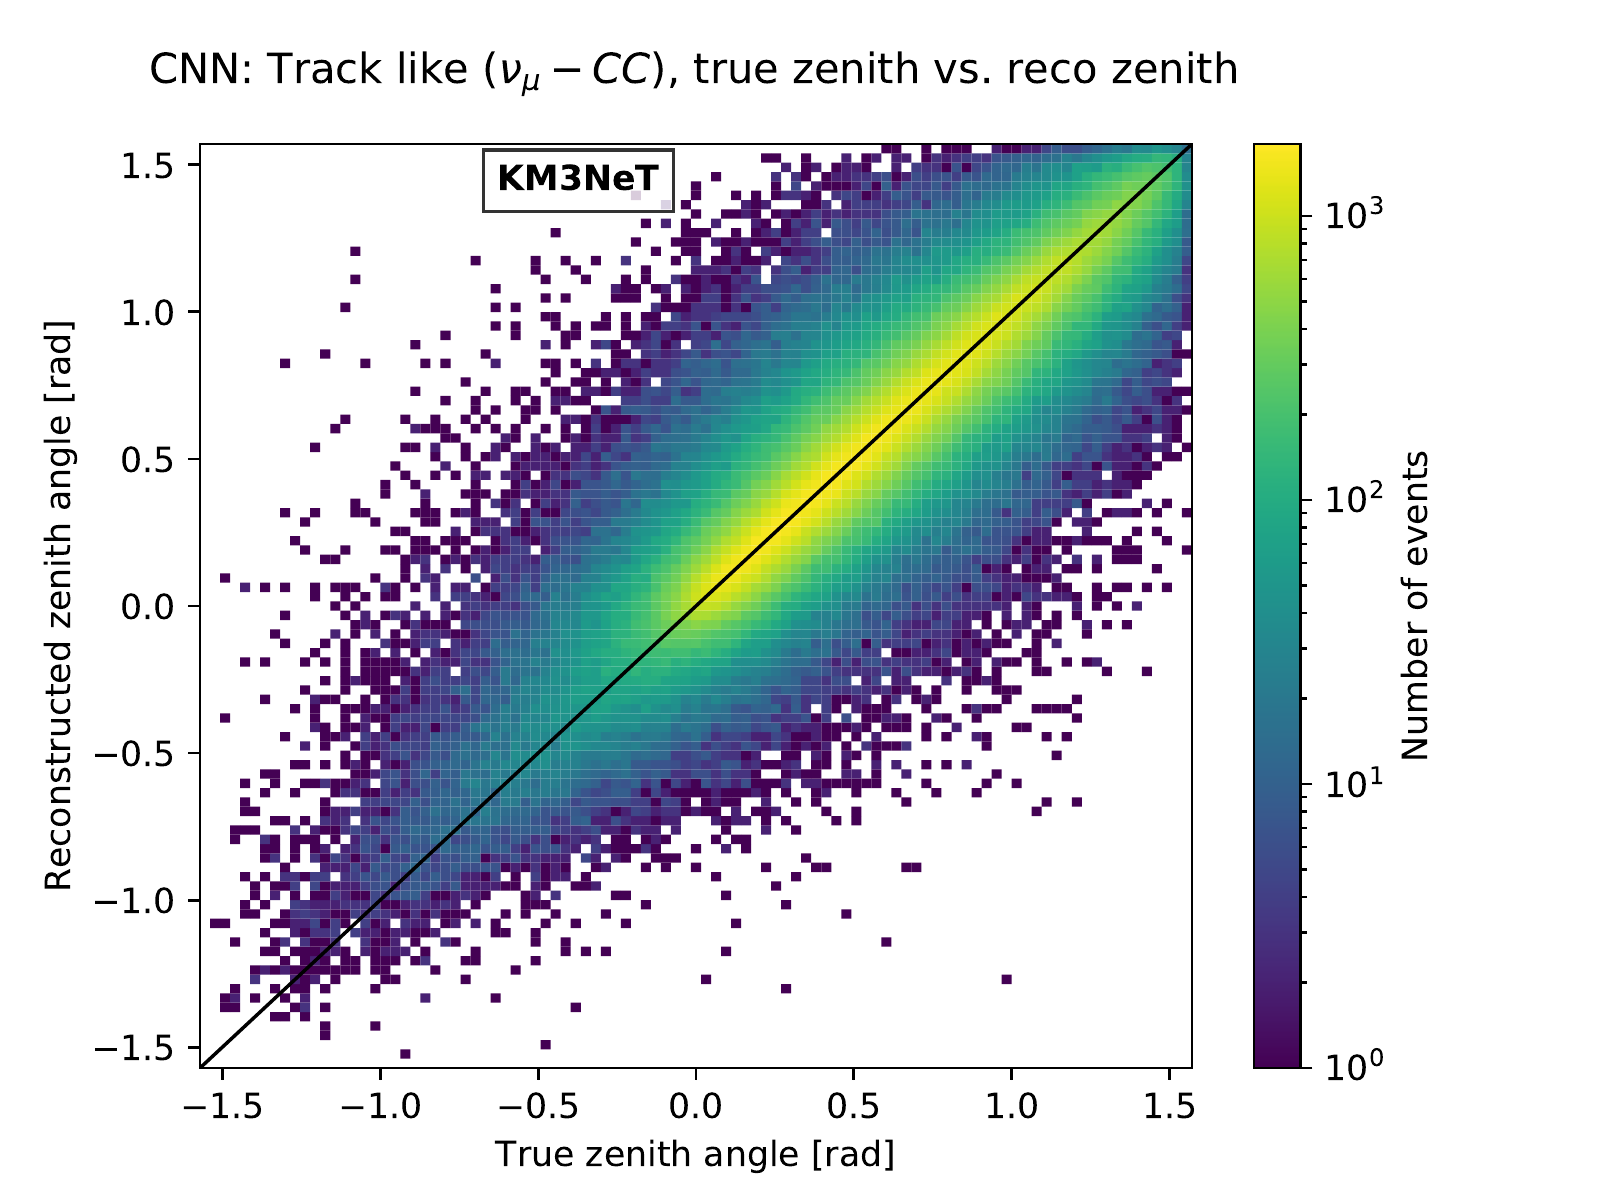}
	\caption{Reconstructed zenith vs. true azimuth of the deep learning reconstruction for $\nu_e-CC$ events. Only events reconstructed as up-going by the standard reconstruction are selected for this plot.}
	\label{fig:regr_2d_zenith_dl_nu_e_cc}
\end{figure}

\begin{figure}[h!]
	\centering \includegraphics[width=0.675\textwidth, page=2]{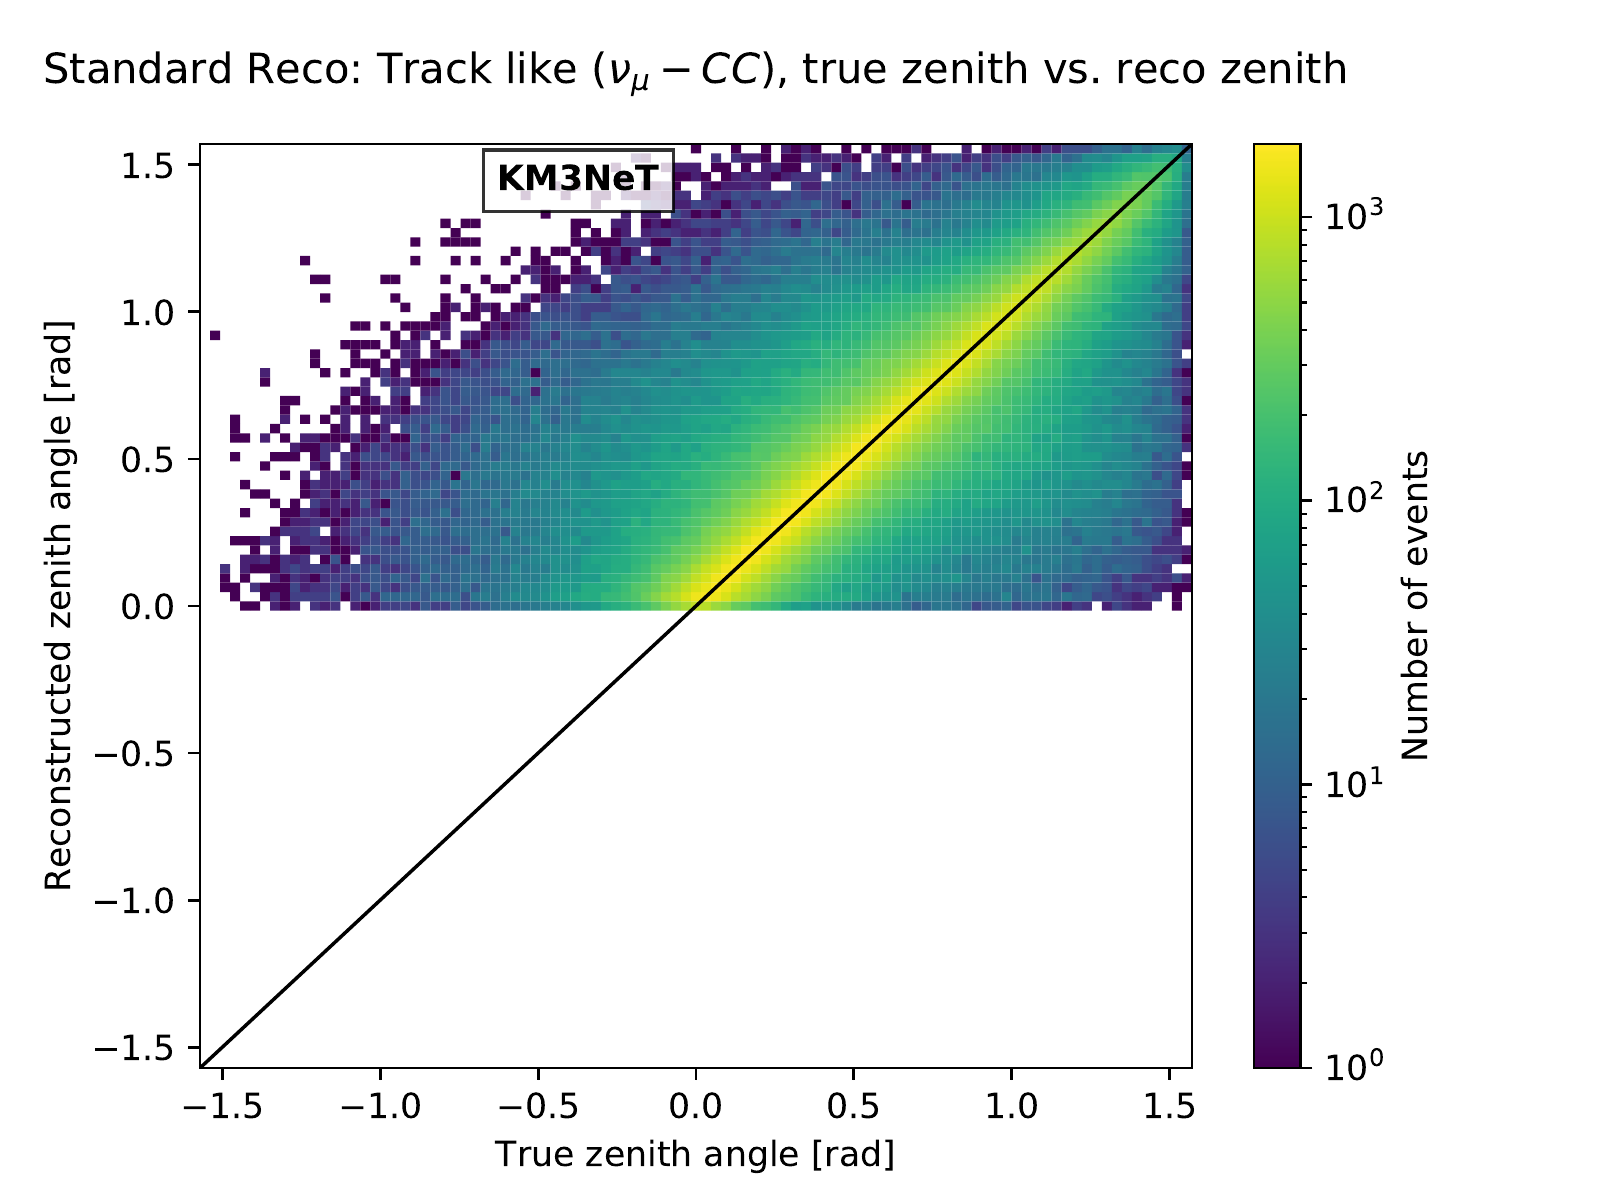}
	\caption{Reconstructed zenith vs. true azimuth of the standard, likelihood-based ORCA reconstruction for $\nu_e-CC$ events. Only events reconstructed as up-going by the standard reconstruction are selected for this plot.}
	\label{fig:regr_2d_zenith_std_nu_e_cc}
\end{figure}

\newpage
\clearpage

\subsection{$\nueNC$ events}

% --- DIRECTION RECONSTRUCTION NU_E_NC

$\nu_e-NC$ azimuth:

\begin{figure}[h!]
	\centering \includegraphics[width=0.675\textwidth, page=3]{img/regression/dir/azimuth_true_to_azimuth_reco.pdf}
	\caption{Reconstructed azimuth vs. true azimuth of the deep learning reconstruction for $\nu_e-NC$ events.}
	\label{fig:regr_2d_azimuth_dl_nu_e_nc}
\end{figure}

\begin{figure}[h!]
	\centering \includegraphics[width=0.675\textwidth, page=3]{img/regression/dir/standard_reco_azimuth_true_to_azimuth_reco.pdf}
	\caption{Reconstructed azimuth vs. true azimuth of the standard, likelihood-based ORCA reconstruction for $\nu_e-NC$ events.}
	\label{fig:regr_2d_azimuth_std_nu_e_nc}
\end{figure}
\newpage
\clearpage

$\nu_e-NC$ zenith:

\begin{figure}[h!]
	\centering \includegraphics[width=0.675\textwidth, page=3]{img/regression/dir/zenith_true_to_zenith_reco.pdf}
	\caption{Reconstructed zenith vs. true azimuth of the deep learning reconstruction for $\nu_e-NC$ events. Only events reconstructed as up-going by the standard reconstruction are selected for this plot.}
	\label{fig:regr_2d_zenith_dl_nu_e_nc}
\end{figure}

\begin{figure}[h!]
	\centering \includegraphics[width=0.675\textwidth, page=3]{img/regression/dir/standard_reco_zenith_true_to_zenith_reco.pdf}
	\caption{Reconstructed zenith vs. true azimuth of the standard, likelihood-based ORCA reconstruction for $\nu_e-NC$ events. Only events reconstructed as up-going by the standard reconstruction are selected for this plot.}
	\label{fig:regr_2d_zenith_std_nu_e_nc}
\end{figure}

\newpage
\clearpage

$\nu_e-NC$ ME:

\begin{figure}[h!]
	\centering \includegraphics[width=0.675\textwidth, page=3]{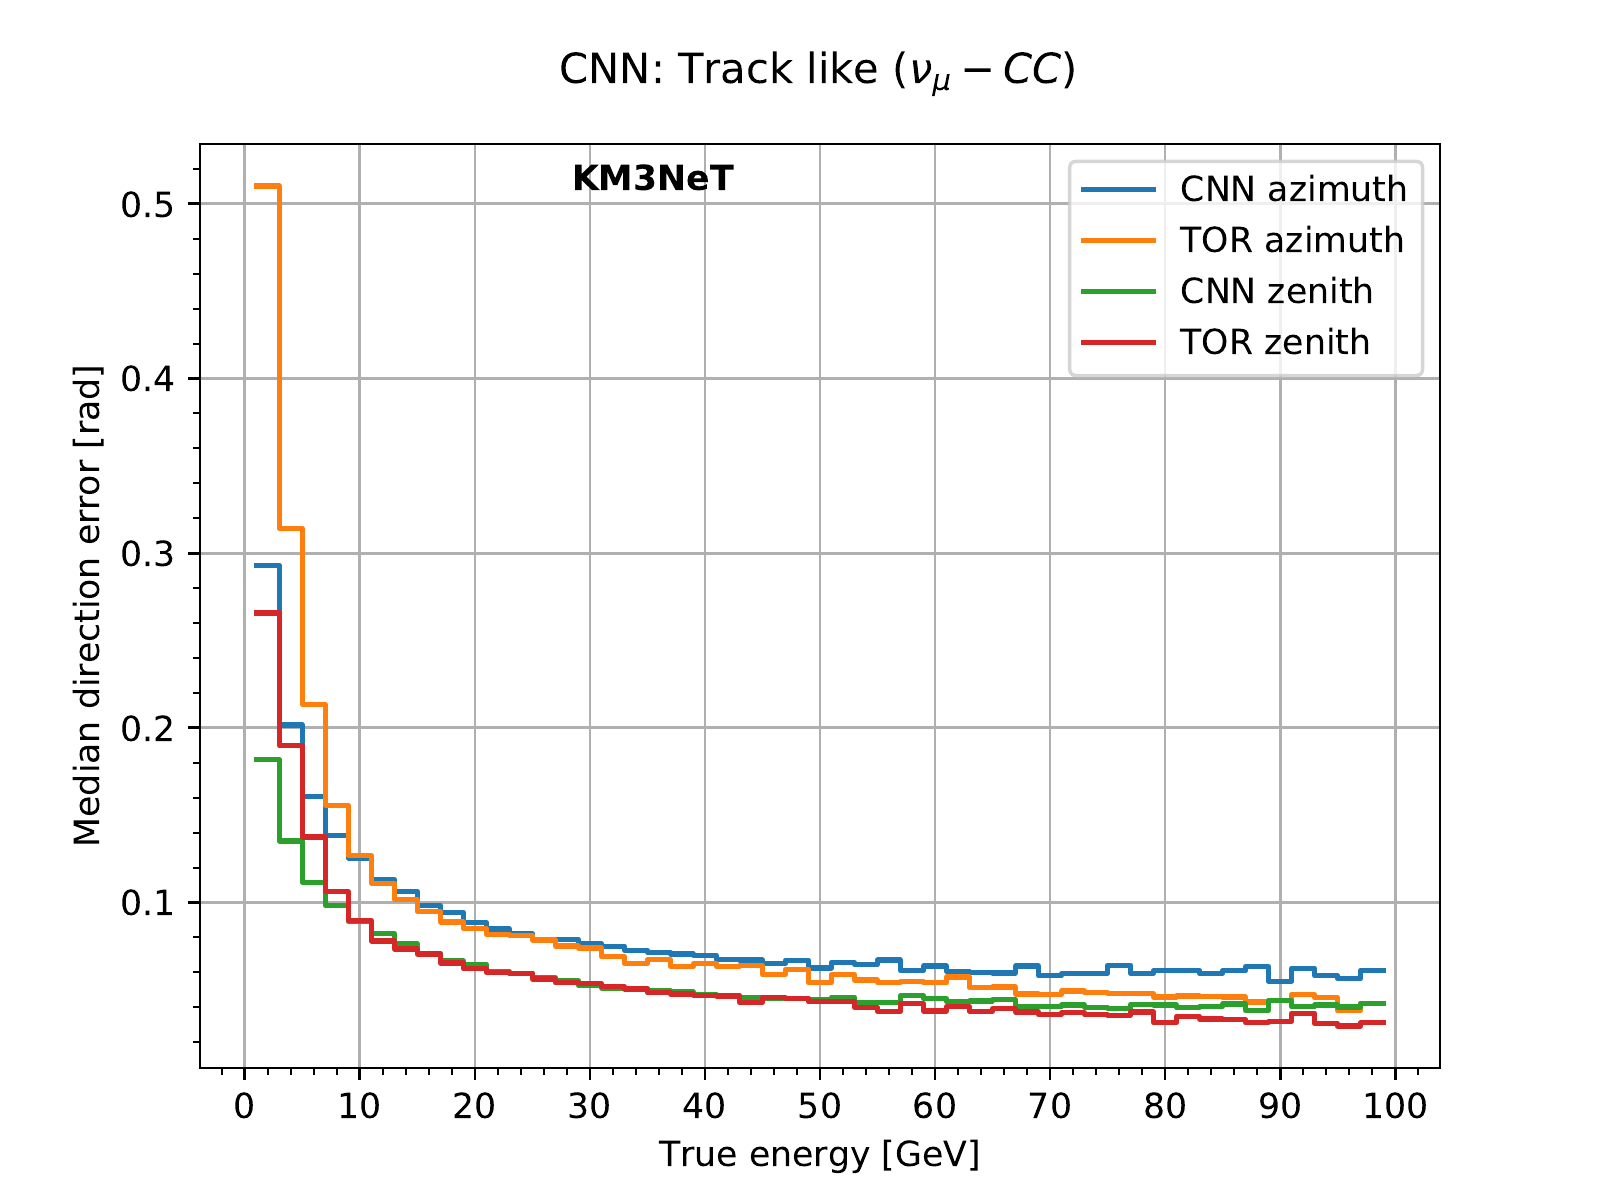}
	\caption{True energy versus the median relative error for $\nu_e-NC$ events and both the deep learning as well as the standard likelihood-based approach.}
	\label{fig:regr_1d_azimuth_nu_e_nc_median}
\end{figure}
