# Supplementary material for: Event reconstruction for KM3NeT/ORCA using convolutional neural networks
Source: arXiv:2004.08254 source file (2020-04-17)
Supplement: Supplementary file 2 [file cnn_appendix_internal.tex]

\section{Extended overview on convolutional neural networks for KM3NeT reviewers}

This appendix section features a small (!) introduction to
Convolutional Neural Networks (CNN) for Deep Learning (DL)
newcomers. If you're starting from zero, you'll probably still feel a
little bit lost after reading this section. Thus, it is recommended to read
http://cs231n.github.io/convolutional-networks as well. \\

Convolutional neural networks form a specialized class of deep neural
networks.  Generally, neural networks are used in order to approximate
a function $f(x)$, which maps from a certain number of inputs $x_i \in
X$ to some outputs $y_i \in Y$.  Then, the goal is to find an
approximation $\hat{f}(x)$ to the function $f(x)$ that describes the
relationship between the inputs $x_i$ and the outputs $y_i$.  Neural
networks are based on the concept of artificial "neurons" that are
arranged in layers. For a fully connected neural network, each neuron
in layer $l$ is connected to each neuron in layer $l-1$. The number
of neurons inside of a layer determines the \textbf{width} of the
network and the number of layers the \textbf{depth} of a network.
Stacking multiple layers of neurons can be interpreted as multiple
functions that are acting on the input $X$ in a chain. For a two layer
model and thus two functions $f^{(1)}$ and $f^{(2)}$ we get (the "hat"
of $\hat{f}$ is neglected from this point on):
\begin{equation*}
f(x) = f^{(2)}(f^{(1)}(x))
\end{equation*}

\begin{figure}[h!]
	\centering
	%\captionsetup{justification=centering}
	\includegraphics[width=0.6\textwidth]{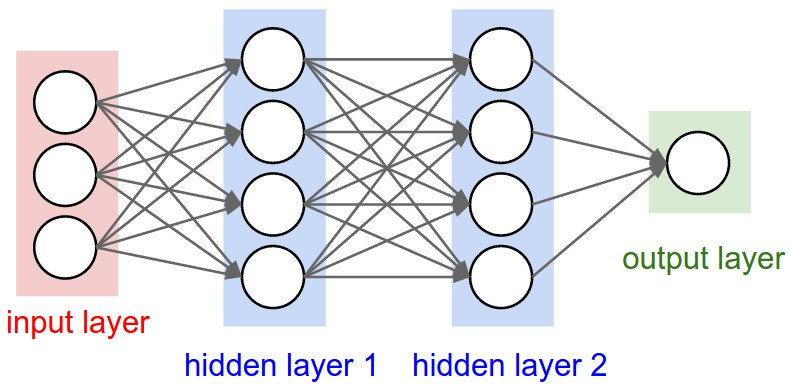}
	\caption[Scheme of a fully connected neural network with two hidden layers and four neurons per hidden layer.]{Scheme of a fully connected neural network with two hidden layers and four neurons per hidden layer.} %\autocite{StanfordUniversity}}
	\label{fig:fc_1_scheme}
\end{figure}

Here, $f^{(1)}$ refers to the first layer in the network and $f^{(2)}$
to the second. The first layer of a neural network is called the
\textbf{input} layer, the intermediate layers are called the
\textbf{hidden} layers and the last layer is called the
\textbf{output} layer.

In order to learn the relationship between $(X,Y)$, learnable weights
are used for each neuron. Suppose we have a single neuron with inputs
$x_i$, then each input $x_i$ of the neuron has a weight $w_i$
associated to this input. Additionally, a single, learnable
\textbf{bias} parameter is added in order to increase the flexibility
of the model to fit the data. This process in a neuron, consisting of
the weights $w_i$ and the bias $b$ is called the \textbf{transfer
  function}:
\begin{equation*}
f_\Sigma = \sum_{i=1}^{n}w_i x_i + b
\end{equation*}

Based on this equation, it can be seen that the response of the neuron
to the input is a linear one. However, many physical processes in
nature are inherently nonlinear. For this reason, one can wrap the
output of the transfer function in another, nonlinear function. It can
be shown that a non-linear 2 layer neural network can approximate any
function.

Nowadays, the most commonly used function is the \textbf{rectified
  linear unit} (ReLU):
\begin{equation*}
f_{\text{ReLU}}(x) = \max (0,x)
\end{equation*}
Such a function is called the \textbf{activation} function.

Now, the weights of each neuron get updated iteratively during a
so-called training process. For this purpose, one needs to define a
so-called cost or loss function, which measures the distance between
the output of the neural network $\hat{f}(x) = \hat{y}$ and the ground
truth $y_{\text{true}}$. This can e.g. be done by measuring the mean
squared error (MSE) and minimizing $(y_{\text{true}}-\hat{f}(x))^2$.
However, since the neural network uses nonlinear activations, most
cost functions, like the mean squared error, become non-convex. Hence,
convex optimization algorithms that guarantee the convergence of the
training with any starting condition cannot be used. Thus, typically
iterative, gradient descent based optimization algorithms are used
that minimize the cost function until a low value is achieved. During
this training process, the cost error is back propagated using the
back-propagation algorithm, which allows for the tuning of the neural
networks' weights.

CNNs are typically used in domains, where the input can be expected to
be image-like, i.e. in image or video classification.  In this regard,
several changes are made in the architecture of CNNs compared to fully
connected neural networks. The main concepts of convolutional neural
networks are based on only locally and not fully connected networks
and on parameter sharing between certain neurons in the network.

Suppose that we have 2D images as the input of our convolutional
neural network. Since most images are colored, they are actually three
dimensional: width, height and channel. Here, the channel dimension
specifies the brightness for each color channel (red, green and blue)
of the image. This three dimensional tensor is then used as an input
for the first convolutional layer.

\begin{figure}[h!]
	\centering
	\includegraphics[width=0.5\textwidth]{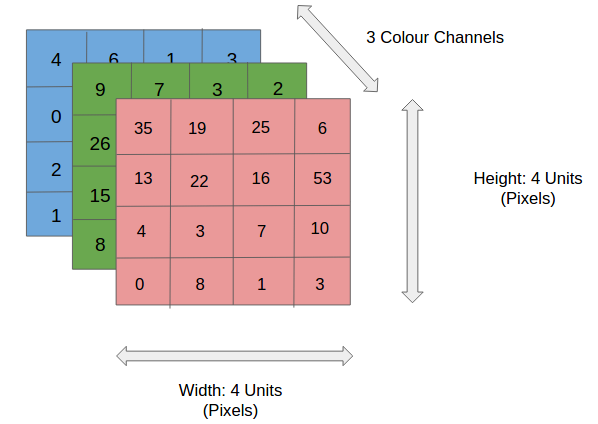}
	\caption[Representation of a $4\times4$ RGB image as a three dimensional array.]{Representation of a $4\times4$ RGB image as a three dimensional array. The brightness of each channel is indicated with numbers ranging from 0 to 255.}
	\label{fig:image_channels}
\end{figure}

Similar to the input layer, the neurons in a convolutional layer are
also arranged in three dimensions: width, height and depth.  One of
the main differences between convolutional layers and fully connected
layers is that the neurons inside a convolutional layer are only
connected to a local region of the input volume. This is often called
the "receptive field" or also the "kernel size" of the neuron.  The
connections of this local area to the neuron are be local in space
(width, height), but they are always full along the depth of the input
volume. Hence, if we have a $[32\times32\times3]$ image (width,
height, channel) and kernel size 5, each neuron in the first
convolutional layer would be connected to a local $[5\times5\times3]$
(width, height, depth) patch of the input. And for each of these
connections, a weight is assigned, such that each neuron has a [$5
  \times 5 \times 3$] weight matrix, which is often called the
"kernel". These weights are now used in performing a dot product
between the receptive field of the neuron and its associated
kernel. Here, the total number of parameters for the single neuron
would be $5 \cdot 5 \cdot 3 + 1 ~(\text{bias}) = 76$. Additionally,
each neuron at the same depth level covers a different part of the
image with its receptive field.

\begin{figure}[h!]
	\centering
        \includegraphics[width=0.75\textwidth]{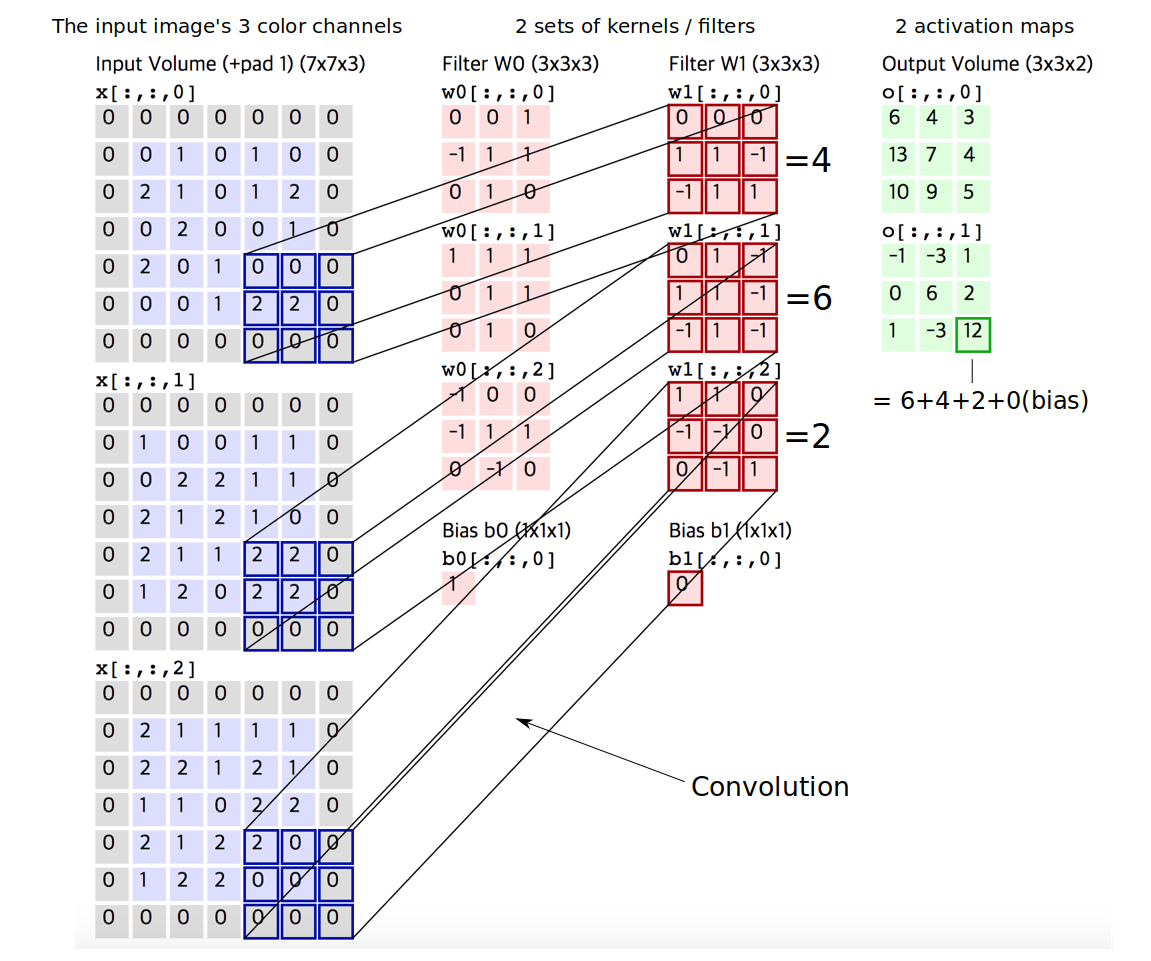}
	\caption{Visualization of computing the dot product
          between the $[3\times3]$ filter (kernel) $W_1$ and the $[7\times7\times3]$ input volume. } %\autocite{image_channels_2016}}
	\label{fig:conv_scheme_1}
\end{figure}

For CNNs, the assumption is now made that a feature at position $(x_1,
y_1)$ could also be useful at another position $(x_2, y_2)$. Under
this assumption, the neurons in a certain depth slice can share their
weights, which significantly reduces the number of parameters in the
network.

\begin{figure}[h!]
	\centering
        \includegraphics[width=0.8\textwidth]{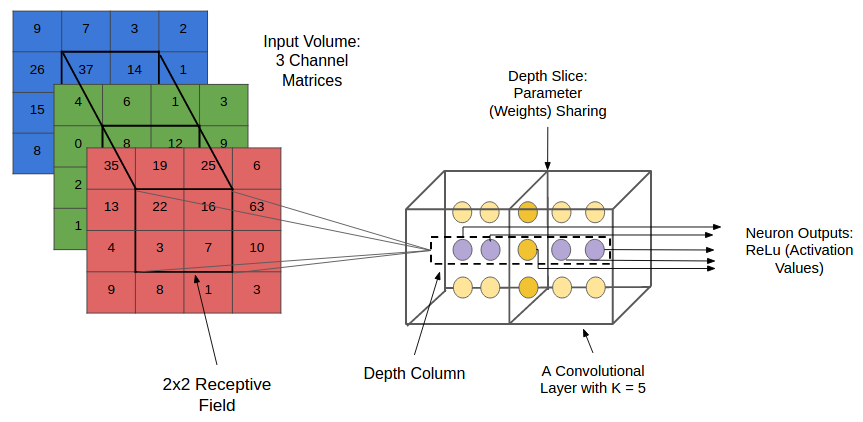}
	\caption[Concept of the depth slice and the receptive field in
          a convolutional layer.]{Concept of the depth slice and the
          receptive field in a convolutional layer.}
        %\autocite{image_channels_2016}}
	\label{fig:depth_slice}
\end{figure}

Usually, between some convolutional layers of a CNN, the number of
parameters is further reduced by pooling the input, which reduces the
dimensionality.  Then, the convolutional layers are stacked on each
other, in order to get a basic convolutional neural network. After the
last convolutional layer, a small fully connected network can be added
in order to connect the outputs of the last convolutional layer to the
output neurons of the total network. Instead of the fully connected
neural network, a global average pooling layer is also often used
nowadays.

\begin{figure}[h!]
	\centering
        \includegraphics[width=0.8\textwidth]{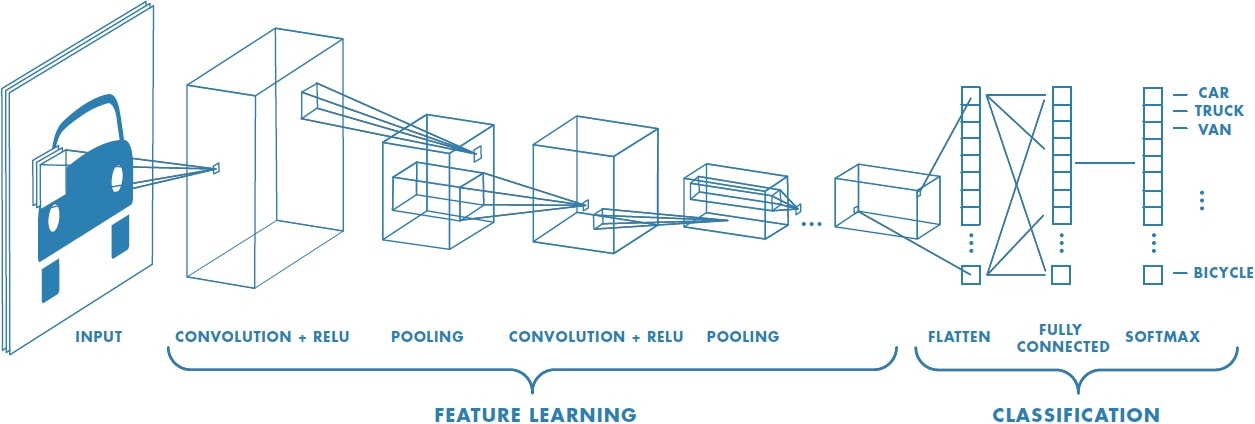}
	\caption[Scheme of a simple convolutional neural
          network.]{Scheme of a simple convolutional neural network. }
        %\autocite{MathWorks_1}}
	\label{fig:cnn_scheme_1}
\end{figure}
